# Supplementary material for: 3DFeat-Net: Weakly Supervised Local 3D Features for Point Cloud Registration
Source: arXiv:1807.09413 ancillary file (2018-07-25)
Supplement: Supplementary file 1 [file supplementary.pdf]

# 3DFeat-Net: Weakly Supervised Local 3D Features for Point Cloud Registration - Supplementary Material

Zi Jian Yew and Gim Hee Lee

Department of Computer Science, National University of Singapore  
{zijian.yew, gimhee.lee}@comp.nus.edu.sg

## 1 Detailed Results for ETH dataset

In this section, we show detailed results on the ETH “challenging dataset for point cloud registration algorithms” [7]. As in [1], we evaluate on the Gazebo and Wood scenes which are each captured in two different seasons (Table 1). Each season-scene combination has its respective coordinate frame, and groundtruth poses are available to relate the local point clouds within the same season and scene. We use these groundtruth poses to stitch all the individual point clouds to generate four global point clouds, one for each season-scene combination.

**Table 1.** ETH Dataset breakdown

| Scene  | Season Pairs   |
|--------|----------------|
| Gazebo | Summer, Winter |
| Wood   | Summer, Autumn |

We note that the ground truth transformations between two different seasons of the same scene are not provided in the original dataset. We circumvent this problem via manual registration of the global point clouds. We get the following transformations for Gazebo:

$$T_{\text{summer} \leftarrow \text{winter}} = \begin{bmatrix} 1 & 0 & 0 & 0.6 \\ 0 & 1 & 0 & 0.3 \\ 0 & 0 & 1 & 0 \\ 0 & 0 & 0 & 1 \end{bmatrix}, \quad (1)$$

and Wood:

$$T_{\text{summer} \leftarrow \text{autumn}} = \begin{bmatrix} \cos 10^\circ & \sin 10^\circ & 0 & -0.2 \\ -\sin 10^\circ & \cos 10^\circ & 0 & 0 \\ 0 & 0 & 1 & 0 \\ 0 & 0 & 0 & 1 \end{bmatrix}. \quad (2)$$

We evaluate our approach by registering winter local point clouds to the summer global point cloud for the Gazebo scene, and autumn local point clouds to the summer global point cloud for the Wood scene. The performance for this dataset is evaluated as per [1], i.e. point clouds registered to within 1m are considered successful. RTE and RRE values are computed for the successful registrations. There are 31 and 32 local point clouds for Gazebo winter and Wood autumn scenes respectively. Table 2 summarizes the statistics computed over the *entire* dataset, with the detailed breakdown shown in Fig. 1. 3DFeat-Net outperforms most algorithms in all measures except USC which uses a 1,980-dimensional descriptor.

**Table 2.** Performance on the entire ETH dataset

| Method                  | RTE (m)                             | RRE ( $^{\circ}$ )                | Success Rate |
|-------------------------|-------------------------------------|-----------------------------------|--------------|
| ISS [11] + SI [4]       | $0.332 \pm 0.197$                   | $5.93 \pm 5.20$                   | 93.7%        |
| ISS [11] + USC [9]      | <b><math>0.223 \pm 0.148</math></b> | <b><math>3.11 \pm 1.80</math></b> | <b>100%</b>  |
| ISS [11] + CGF [5]      | $0.290 \pm 0.193$                   | $5.31 \pm 5.63$                   | 92.1%        |
| RS + 3DMatch [10]       | $0.414 \pm 0.275$                   | $14.94 \pm 28.25$                 | 33.3%        |
| ISS [11] + 3DMatch [10] | $0.530 \pm 0.266$                   | $17.41 \pm 22.11$                 | 33.3%        |
| <b>Our Kpt + Desc</b>   | $0.277 \pm 0.171$                   | $4.45 \pm 3.84$                   | 95.2%        |

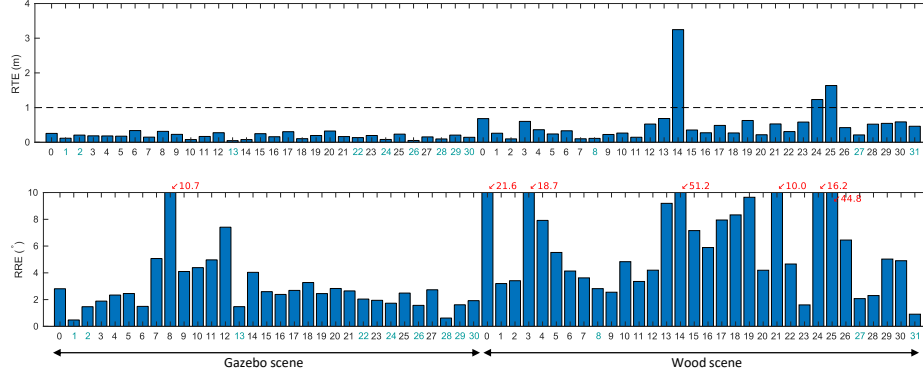

**Fig. 1.** Individual RTE and RRE for the ETH dataset for 3DFeat-Net. Horizontal dashed line in the top plot indicates the 1m threshold for computing binary success. For clarity, the y-axis for the RRE plot is truncated for outliers with the actual value shown in red. Numbers in teal indicate the 12 datasets considered in the main paper.

## 2 Oxford RobotCar Dataset

### 2.1 Data Split

The Oxford RobotCar [6] dataset contains 40 traversals after excluding traversals with bad GPS/INS readings. We split the data into disjoint training and testing sets as shown in Table 3 and Fig. 2.

**Table 3.** Train and test split for Oxford RobotCar dataset.

|                        | Traversals 1-35 | Traversals 36-40 |
|------------------------|-----------------|------------------|
| Northern region (blue) | Training        | Unused           |
| Southern region (red)  | Unused          | Testing          |

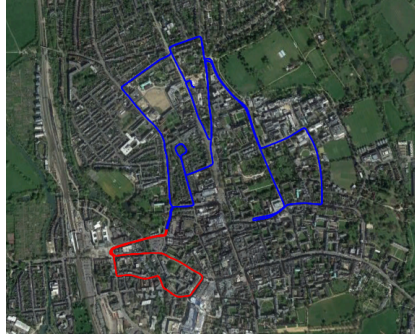

**Fig. 2.** Regions used for training (blue) and testing (red).

### 2.2 GPS/INS Errors

We observe errors of up to around 5 meters when using GPS/INS poses to align the point clouds (Fig. 3). Such large errors makes it difficult to infer accurate point correspondences for strongly supervised training.

## 3 Indoor Performance

We also show the performance of our Feat3D-Net descriptor on the indoor SceneNN [3] dataset in Fig. 4. As in [5], we consider the precision of the feature descriptor over all points. We do not fine-tune our network, but reduce the cluster size  $r_{cluster}$  to 0.35m (obtained from validation) to accommodate the smaller scene. Despite not being trained on indoor datasets, our Feat3D-Net obtains competitive performance and performs just slightly worse than the best performing traditional descriptor (USC) which uses a 1,980-dimensional descriptor.

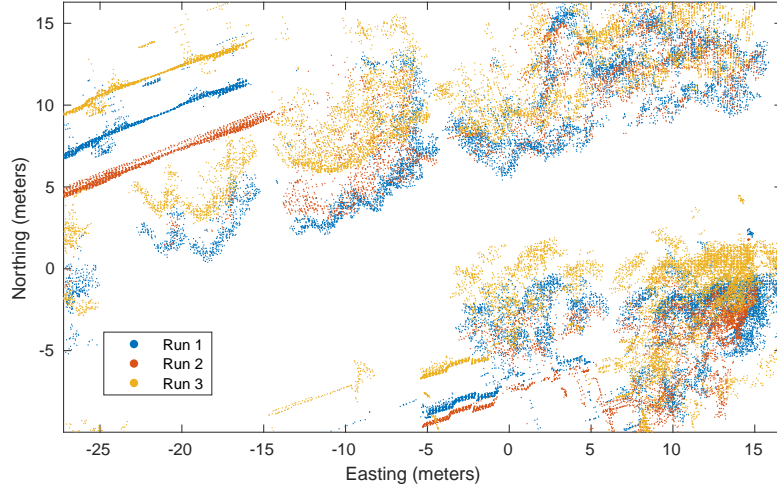

**Fig. 3.** Misalignment of point clouds from different trajectories (Oxford dataset).

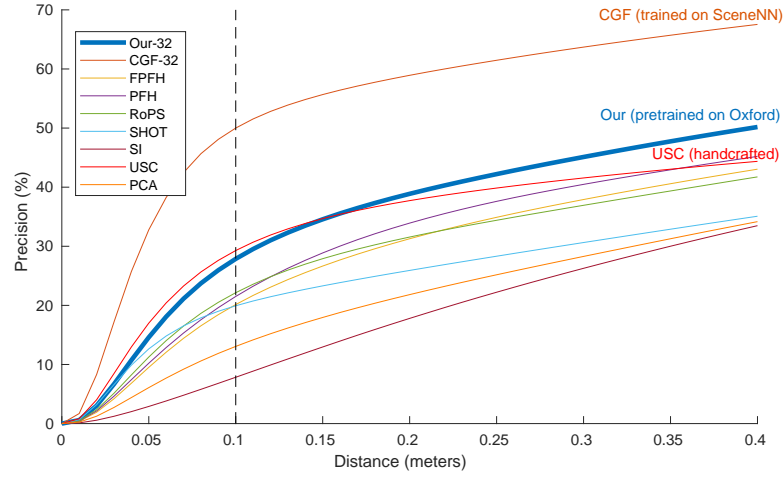

**Fig. 4.** Performance on SceneNN [3] dataset. Baseline results from [5].

## 4 Parameters

Batch normalization and ReLU activation are used for all intermediate layers. We use the softplus activation for the output of the attention, and do not use any activation functions for the final layers that output the orientation and descriptor. We use the same number of nodes for all layers to evaluate the effect of descriptor dimensionality (Fig. 2 in the main paper), except for the last two feature description layers where we use  $d' = 128$  (for output dimension  $d \leq 64$ ) or  $d' = 256$  (for  $d = 128$ ). We also show the parameters used for all baseline algorithms in Table 4. Note that the ISS detector had to be tuned separately for the ETH dataset to obtain good performance.

**Table 4.** Baseline Algorithm Parameters. Parameters not listed are set to their default values in PCL [2].

| Algorithm                   | Parameter                                        | Value          |
|-----------------------------|--------------------------------------------------|----------------|
| ISS [11]<br>(Oxford, KITTI) | Saliency radius ( $r_{salient}$ )                | 1.0            |
|                             | Non-max suppression radius ( $r_{nms}$ )         | 0.5            |
|                             | Saliency thresholds $[\gamma_{21}, \gamma_{32}]$ | [0.975, 0.975] |
|                             | Min neighbors                                    | 7              |
| ISS [11]<br>(ETH)           | Saliency radius ( $r_{salient}$ )                | 1.0            |
|                             | Non-max suppression radius ( $r_{nms}$ )         | 0.2            |
|                             | Saliency thresholds $[\gamma_{21}, \gamma_{32}]$ | [0.975, 0.975] |
|                             | Min neighbors                                    | 5              |
| USC [9]                     | Min Radius $r_{min}$                             | 0.1            |
|                             | RF radius $r_{local}$                            | 4.0            |
|                             | Density radius ( $\delta$ )                      | 1.0            |
| SI [4]                      | Search radius ( $r$ )                            | 4.0            |
| FPFH [8]                    | Search radius ( $r$ )                            | 4.0            |
| 3DMatch [10]                | Voxel size                                       | 0.13 cm        |
| CGF [5]                     | Search radius ( $r$ )                            | 4.0            |

## 5 Additional Qualitative Results

We show additional qualitative registration results by our approach in Fig. 5 and 6, including a failure case for the Oxford RobotCar dataset due to lack of sufficient distinctive local features.

Oxford RobotCar

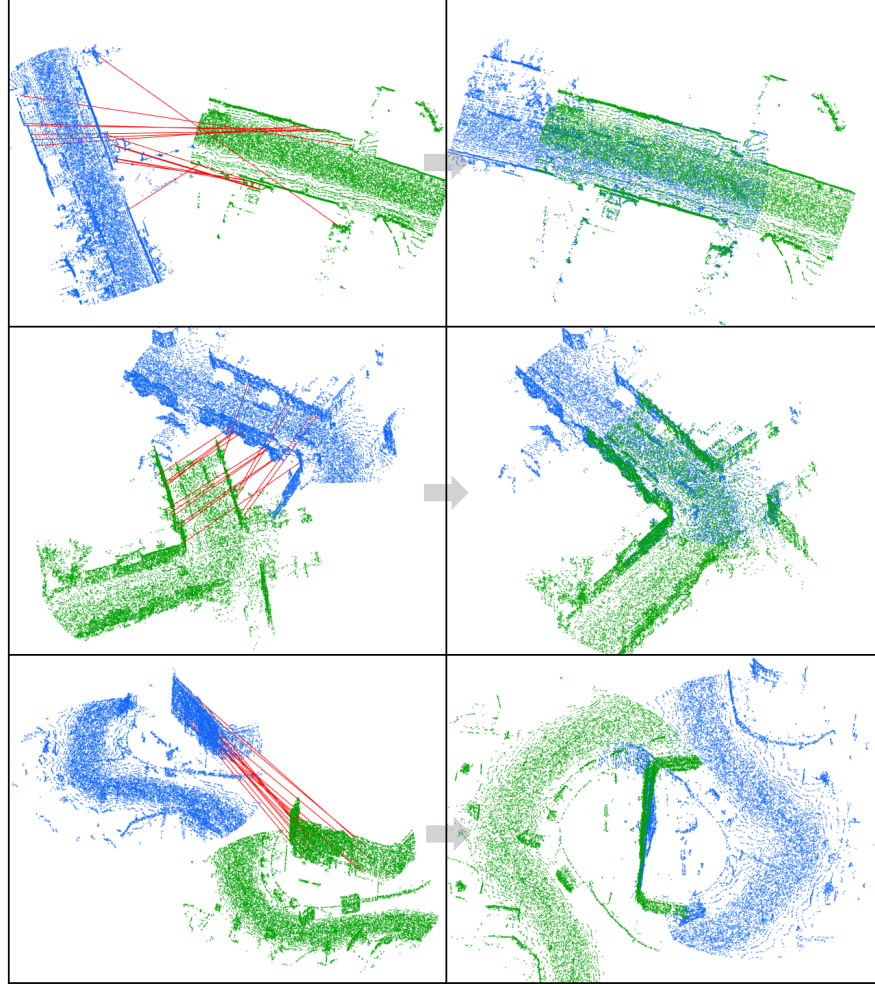

**Fig. 5.** Additional registration results by our approach for Oxford Robotcar dataset. The third row shows an example of a failure case due to the building's symmetry and lack of good local textures. ISS+FPFH fails for all of these cases.

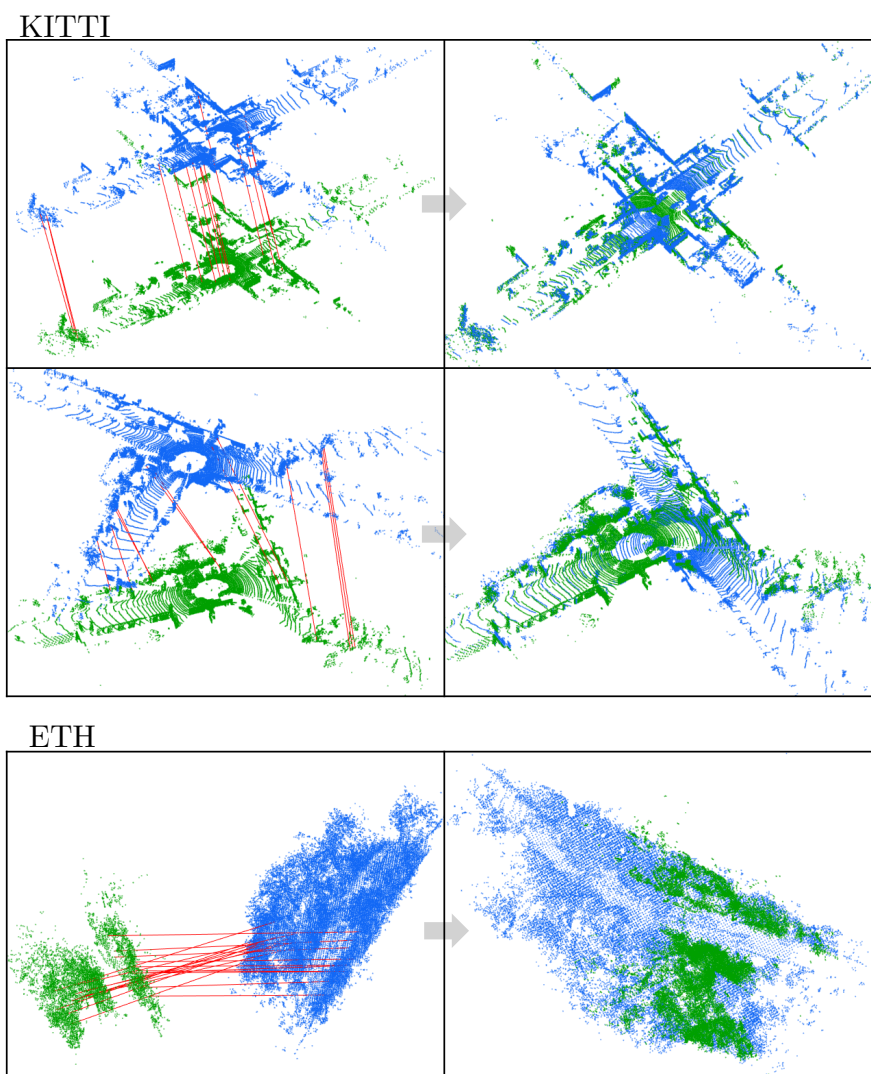

**Fig. 6.** Additional registration results by our approach for KITTI and ETH (Wood) datasets. Top portion of ETH dataset is truncated for ease of visualization. ISS+FPFH fails for all of these cases.

## References

1. Elbaz, G., Avraham, T., Fischer, A.: 3d point cloud registration for localization using a deep neural network auto-encoder. In: IEEE Conference on Computer Vision and Pattern Recognition (CVPR). pp. 2472–2481 (2017). <https://doi.org/10.1109/CVPR.2017.265>
2. Holz, D., Ichim, A.E., Tombari, F., Rusu, R.B., Behnke, S.: Registration with the point cloud library: A modular framework for aligning in 3-d. IEEE Robotics Automation Magazine **22**(4), 110–124 (Dec 2015). <https://doi.org/10.1109/MRA.2015.2432331>
3. Hua, B.S., Pham, Q.H., Nguyen, D.T., Tran, M.K., Yu, L.F., Yeung, S.K.: Scenenn: A scene meshes dataset with annotations. In: International Conference on 3D Vision (3DV). pp. 92–101 (2016). <https://doi.org/10.1109/3DV.2016.18>
4. Johnson, A.E., Hebert, M.: Using spin images for efficient object recognition in cluttered 3d scenes. IEEE Transactions on Pattern Analysis and Machine Intelligence (TPAMI) **21**(5), 433–449 (1999). <https://doi.org/10.1109/34.765655>
5. Khoury, M., Zhou, Q.Y., Koltun, V.: Learning compact geometric features. In: International Conference on Computer Vision (ICCV). pp. 153–161 (2017). <https://doi.org/10.1109/ICCV.2017.26>
6. Maddern, W., Pascoe, G., Linegar, C., Newman, P.: 1 year, 1000km: The oxford robotcar dataset. The International Journal of Robotics Research (IJRR) **36**(1), 3–15 (2017). <https://doi.org/10.1177/0278364916679498>
7. Pomerleau, F., Liu, M., Colas, F., Siegwart, R.: Challenging data sets for point cloud registration algorithms. The International Journal of Robotics Research (IJRR) **31**(14), 1705–1711 (Dec 2012)
8. Rusu, R.B., Blodow, N., Beetz, M.: Fast point feature histograms (fpfh) for 3d registration. In: IEEE International Conference on Robotics and Automation (ICRA). pp. 3212–3217 (2009). <https://doi.org/10.1109/ROBOT.2009.5152473>
9. Tombari, F., Salti, S., Di Stefano, L.: Unique shape context for 3d data description. In: ACM Workshop on 3D Object Retrieval. pp. 57–62. 3DOR ’10, ACM (2010). <https://doi.org/10.1145/1877808.1877821>
10. Zeng, A., Song, S., Nießner, M., Fisher, M., Xiao, J., Funkhouser, T.: 3dmatch: Learning local geometric descriptors from rgb-d reconstructions. In: IEEE Conference on Computer Vision and Pattern Recognition (CVPR). pp. 199–208 (2017). <https://doi.org/10.1109/CVPR.2017.29>
11. Zhong, Y.: Intrinsic shape signatures: A shape descriptor for 3d object recognition. In: IEEE International Conference on Computer Vision Workshops, (ICCVW). pp. 689–696 (2009). <https://doi.org/10.1109/ICCVW.2009.5457637>
